# Supplementary material for: RoCoDA: Counterfactual Data Augmentation for Data-Efficient Robot Learning from Demonstrations
Source: arXiv:2411.16959 source file (2025-05-20)
Supplement: Supplementary file 1 [file 5-appendix.tex]

\section*{Appendix}

% {\setlength{\parskip}{0pt}
\subsection{Assumptions \& Limitations}
\begin{enumerate}
\item \textbf{Generating demonstrations from human source.} We use the same assumptions as \cite{mandlekar2023mimicgen} to generate new demonstrations.
\item \textbf{Access to simulation states.} We use information about simulation states to create new demonstrations and to create causally augmented data.
\item \textbf{Subtask boundaries are determined by changes in gripper state.} Defining the subtask boundaries by changes in the gripper state limits the the environments we experiment on.  Environments that involve skills such as pushing or pulling objects would require using a different heuristic to divide subtasks.
\item \textbf{Causal Relationships are known.} The causal relationships between entities are assumed to be known by a domain expert. For each subtask, each timestep is labeled with its corresponding causal graph.
% \item \textbf{Access to simulation states.}
\end{enumerate}
% {\setlength{\parskip}{0pt}

\subsection{Additional Related Works}
\paragraph{\textbf{Data Augmentation}} Data augmentation has played a critical role in the success of machine learning models by artificially expanding the size of training datasets and improving model generalization. Early work in this area applied basic transformations such as rotation, scaling, translation, and distortion to image datasets like MNIST \cite{yaeger1996effective},
% simard2003best
laying the groundwork for modern augmentation methods. The success of convolutional neural networks in image classification tasks further highlighted the importance of data augmentation.  AlexNet \cite{krizhevsky2012imagenet} employed random cropping and horizontal flipping to improve image classification performance. Subsequent methods like Cutout \cite{devries2017improved} and Mixup \cite{zhang2017mixup} introduced techniques for robustness to occlusion and linear interpolation between samples, respectively.

\paragraph{\textbf{Generative Data Synthesis}} As generative models continue to gain popularity \cite{rombach2022high,ramesh2021zero}, researchers have found multiple ways to use them to generate synthetic data for robotics. 
GenAug \cite{chen2023genaug} Utilizes generative models like Stable Diffusion to alter textures and generate diverse visual samples, improving model robustness to appearance variations. ROSIE \cite{yu2023scaling} Performs infilling using generative models to complete partially observed states and generate data with diverse backgrounds. SynthER \cite{lu2024synthetic} trains diffusion models on existing datasets to produce synthetic demonstrations, thus increasing the diversity and size of the training data.
While some approaches \cite{lu2024synthetic, mandi2022cacti, tian2024view, wang2024prioritized, zhang2024diffusion} train diffusion models on existing datasets to produce synthetic demonstrations, increasing the diversity and size of the training data, these methods often focus on high-level semantic variations and may not adequately address low-level spurious correlations in state-action relationships. In this work, we establish a framework that leverages explicit causal and geometric augmentations. Exploring generative models as a complementary strategy is left for future work.
\begin{table}[t]
\centering
\scriptsize % or \tiny for even smaller font
\resizebox{.75\columnwidth}{!}{
\begin{tabular}{l r}
    \midrule
    Image resolution & 240x320x3 \\
    Learning rate & 1e-4  \\ %\hline
    Batch size & 16  \\ %\
    \# of Encoder layers & 4  \\ %\hline
    \# of Decoder layers & 7  \\ %\hline
    Feedforward dimensions & 1600  \\ %\hline\textbf{}
    Hidden dimension & 256  \\ %\hline
    \# of Heads & 8  \\ %\hline
    Chunk size & 15  \\ %\hline
    Beta & 10 \\ %\hline
    Dropout & 0.1  \\ %\hline

    % \rowcolor[HTML]{EFEFEF} 
    % - CAR & & & &\\ %\hline
    \midrule
\end{tabular}
    }
\caption{Hyperparameters of ACT \ag{not necessary in main paper. move to appendix/ website}}
% \vspace{2mm}
\label{tab:hyperparams}
% \vspace{-8mm}
\end{table}

\begin{algorithm}[b]
\caption{Offline Causal Augmentation}
\label{alg:offlineCoDA}
\begin{algorithmic}[1]
\Require Dataset of demonstrations $\mathcal{D} = \{\tau_i\}$, where $\tau_i = \{s_t, a_t\}_{t=1}^{T_i}$, causal graphs $\mathcal{G}$ for task.
\State Initialize $\mathcal{D}_{aug} \gets \mathcal{D}$
\For{each trajectory $\tau \in \mathcal{D}$}
    \For{each timestep $t \in [1, T_i]$}
        \State Retrieve causal graph $\mathcal{G}$ for current phase
        \State Identify causally independent partitions
        \Statex \hspace{3em} of entities  in $\mathcal{G}$
        \For{each partition}
            \State Sample a new partition from another
            \Statex \hspace{4.5em} trajectory in the same causal phase
            % \State Replace the object’s state, ensuring causal 
            % \Statex \hspace{4.5em} ensuring causal consistency with the task
            \State Replace the current partition with the  \Statex \hspace{4.5em} new partition
            \State Render new observation            
        \EndFor
    \EndFor
    \State Add augmented $\tau$ to $\mathcal{D}_{aug}$
\EndFor
    \State \Return Augmented dataset $\mathcal{D}_{aug}$
\end{algorithmic}
\end{algorithm}

\begin{figure*}[!t]
    \centering
    % \vspace{-5mm}
    \includegraphics[width=.9\linewidth]{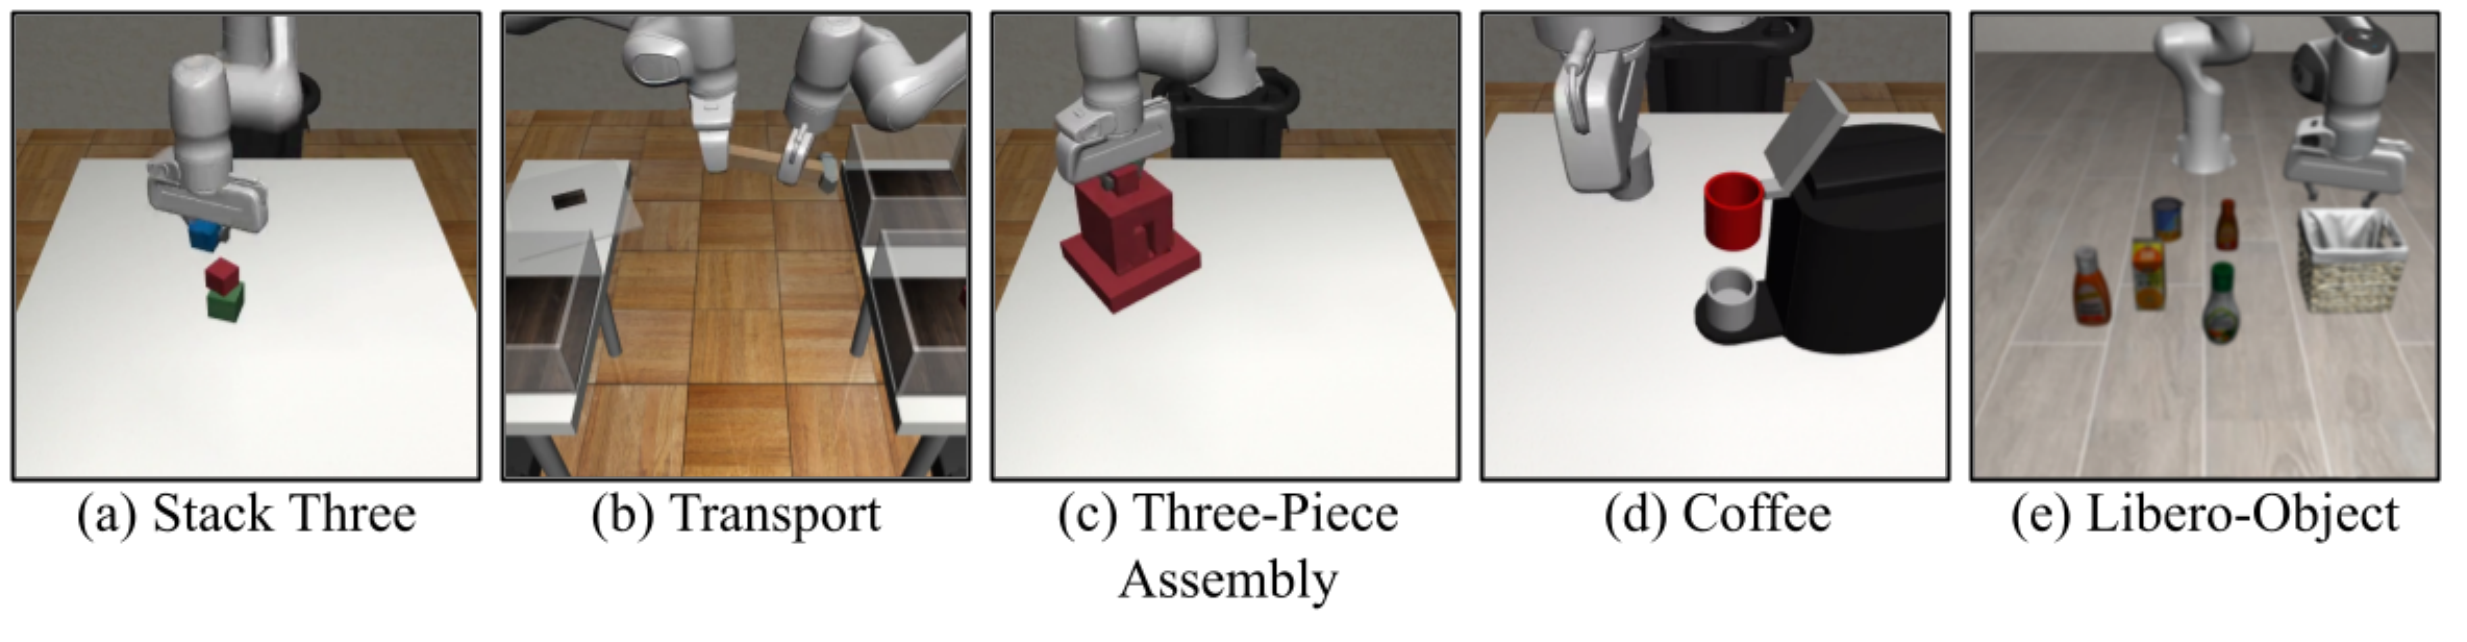}
    \caption{We conduct experiments across five environments, each with a specific goal: \textbf{(a)} stack three blocks in a specified color order, \textbf{(b)} transport a hammer from the left bin to the top-right bin, \textbf{(c)} assemble a structure by connecting pieces in a particular sequence and orientation, \textbf{(d)} place a coffee pod into a coffee maker and close the lid, and \textbf{(e)} pick up a tomato sauce and place it into a basket.}
    \label{fig:environments}
    \vspace{3mm}
\end{figure*}

\subsection{Task Descriptions}
In this section we provide more detail of tasks used in our experiments (Figure \ref{fig:environments}). For our experiments we use a panda arm for data collection and policy rollout. We use source data in collected in \textit{$D_0$} variations of \textit{Three Block Stack}, \textit{Three Piece Assembly} and \textit{Coffee}.

\noindent  \textbf{Three Block Stack:} The robot must stack three distinct colored blocks in order of green, red, and then the blue cube on top. We generate trajectories for the \textit{$D_1$} \cite{mandlekar2023mimicgen} variation of a larger spatial distribution of the blocks on the table.

\noindent \textbf{Three Piece Assembly:} This task requires precision and correct orientation, making it more challenging than simple block stacking due to the importance of part alignment. This task involves building a structure by assembling three pieces in a precise sequence and orientation. We generate trajectories for the \textit{$D_2$} \cite{mandlekar2023mimicgen} variation of the environment where all three pieces have a top-down rotation variation and all pieces can be initialized in different positions. We note that using MimicGen yielded a low success rate of generating trajectories. As MimicGen can generate biased data \cite{mandlekar2023mimicgen} low performance may be due to biased object configurations in the generated dataset.

\noindent \textbf{Coffee Task:} This task tests interaction with articulated objects and sequential dependencies, emphasizing the handling of non-rigid dynamics involving placing a coffee pod into a coffee machine and closing the lid. Different from the source demonstrations the \textit{$D_2$} \cite{mandlekar2023mimicgen} demonstrations have a larger region and rotational variation and the coffee pod and coffee machine initialized positions are switched. 

\noindent \textbf{Libero-Object:} We use a task from the Libero-Object dataset \cite{liu2024libero} where the robot must pick up a specific object (e.g., tomato sauce) and place it in a basket. 
We modify this task during evaluation to measure generalization to unseen objects (distractors), textures, and positions. These experiments were trained with a subset of distractor objects. The evaluations on textures and positions were conducted with the same subset of distractors.

\noindent \textbf{Transport:} This task tests coordination between multiple agents and temporal sequencing. \textit{Transport} \cite{mandlekar2021matters} involves two robotic arms. The left arm removes a lid and picks up a hammer, while the right arm moves a cube from a back bin to a front bin, takes the hammer from the left arm, and places it in another bin. The hammer, cube, bins, and lid each vary slightly in position within a defined region, with the hammer and cube also having variations in rotation. For this task we examine the effect of causal augmentation versus standard augmentation on complex, long-horizon tasks.

\subsection{Causal Relationships for Tasks}
In our experiments, we use spatial information of objects as states to be augmented. In tasks such as block stacking, where the stacking order depends on block color, we could further factorize object states (e.g. color, texture, etc) to enhance augmentation. However, we simplify the causal structure by not factoring object states in this way. We specify causal relationships for each subtask and provide causal graphs for \textit{Three Block Stack} and \textit{Coffee} in Figure \ref{fig:causalstack}. Subtasks are defined based on changes in the robot's gripper state as mentioned in Section \ref{sec:method}. When sampling data, we use the corresponding causal graph to sample new states. For instance, the third phase of \textit{Three Block Stack} has two independent partitions: (1) Robot and Cube C and (2) Cube A and Cube B. As the states of Cube A and B are irrelevant to the robot's movement to Cube C, the states of Cube A and B can be sampled from another trajectory of the same subtask phase without affecting the causal relationship. We additionally factorize the robot's gripper position and augment the gripper position randomly while the robot transits to pick up objects.

% \subsection{Causal Graphs}

\begin{figure}[!b]
    \centering
    % \vspace{-5mm}
    \includegraphics[width=.95\linewidth]{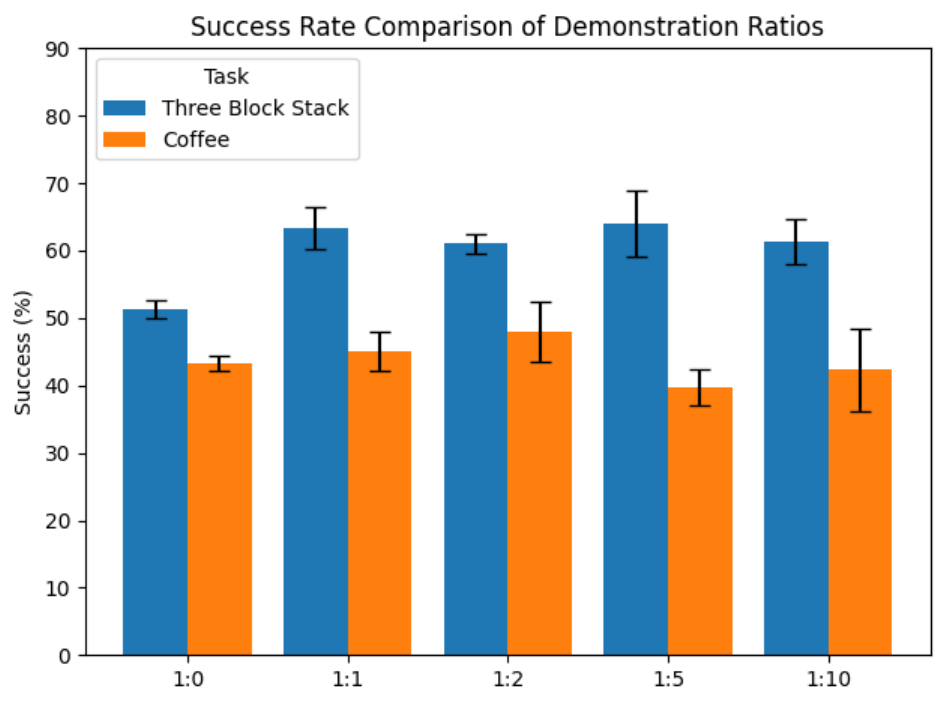}
    \caption{Success Rate vs ratio of demonstration data to synthetic data. The addition of causal augmentation improves performance. As the amount of synthetic data is increased, performance gains diminish.}
    \label{fig:ratio}
    % \vspace{-3mm}
\end{figure}
% {\setlength{\parskip}{0pt}

\subsection{Training Details}
Across all experiments, we keep training hyperparameters unchanged. We use hyperparameters similar to \cite{zhao2023learning}, but decrease the image resolution, feedforward dimensions, and hidden dimensions by a factor of two. We additionally double the batch size and use a chunk size of 15 and do not use temporal ensembling (Table \ref{tab:hyperparams}). We train \textit{Three Block Stack}, \textit{Three Piece Assembly}, and \textit{Coffee} datasets using the \textit{agentview} and \textit{robot0_eye_in_hand} camera views. As for the \textit{Libero Object} dataset, we train on the \textit{agentview} camera view. While for the \textit{Transport} we experiment with single \textit{agentview}  and multicamera view with \textit{robot0_eye_in_hand}, \textit{robot1_eye_in_hand}, \textit{shouldercamera0} and \textit{shouldercamera1} (Table \ref{tab:transportaug}). Similar to \cite{chi2023diffusion}, actions are positional control and use a 6D rotation representation. %For the proprioceptive observation, we use the end-effector position, rotation as a quaternion, and gripper position.

\begin{figure*}[!t]
    \centering
    % \vspace{-5mm}
     \subfloat[Causal Graph of Three Block Stack]{%
        \includegraphics[width=.90\linewidth]{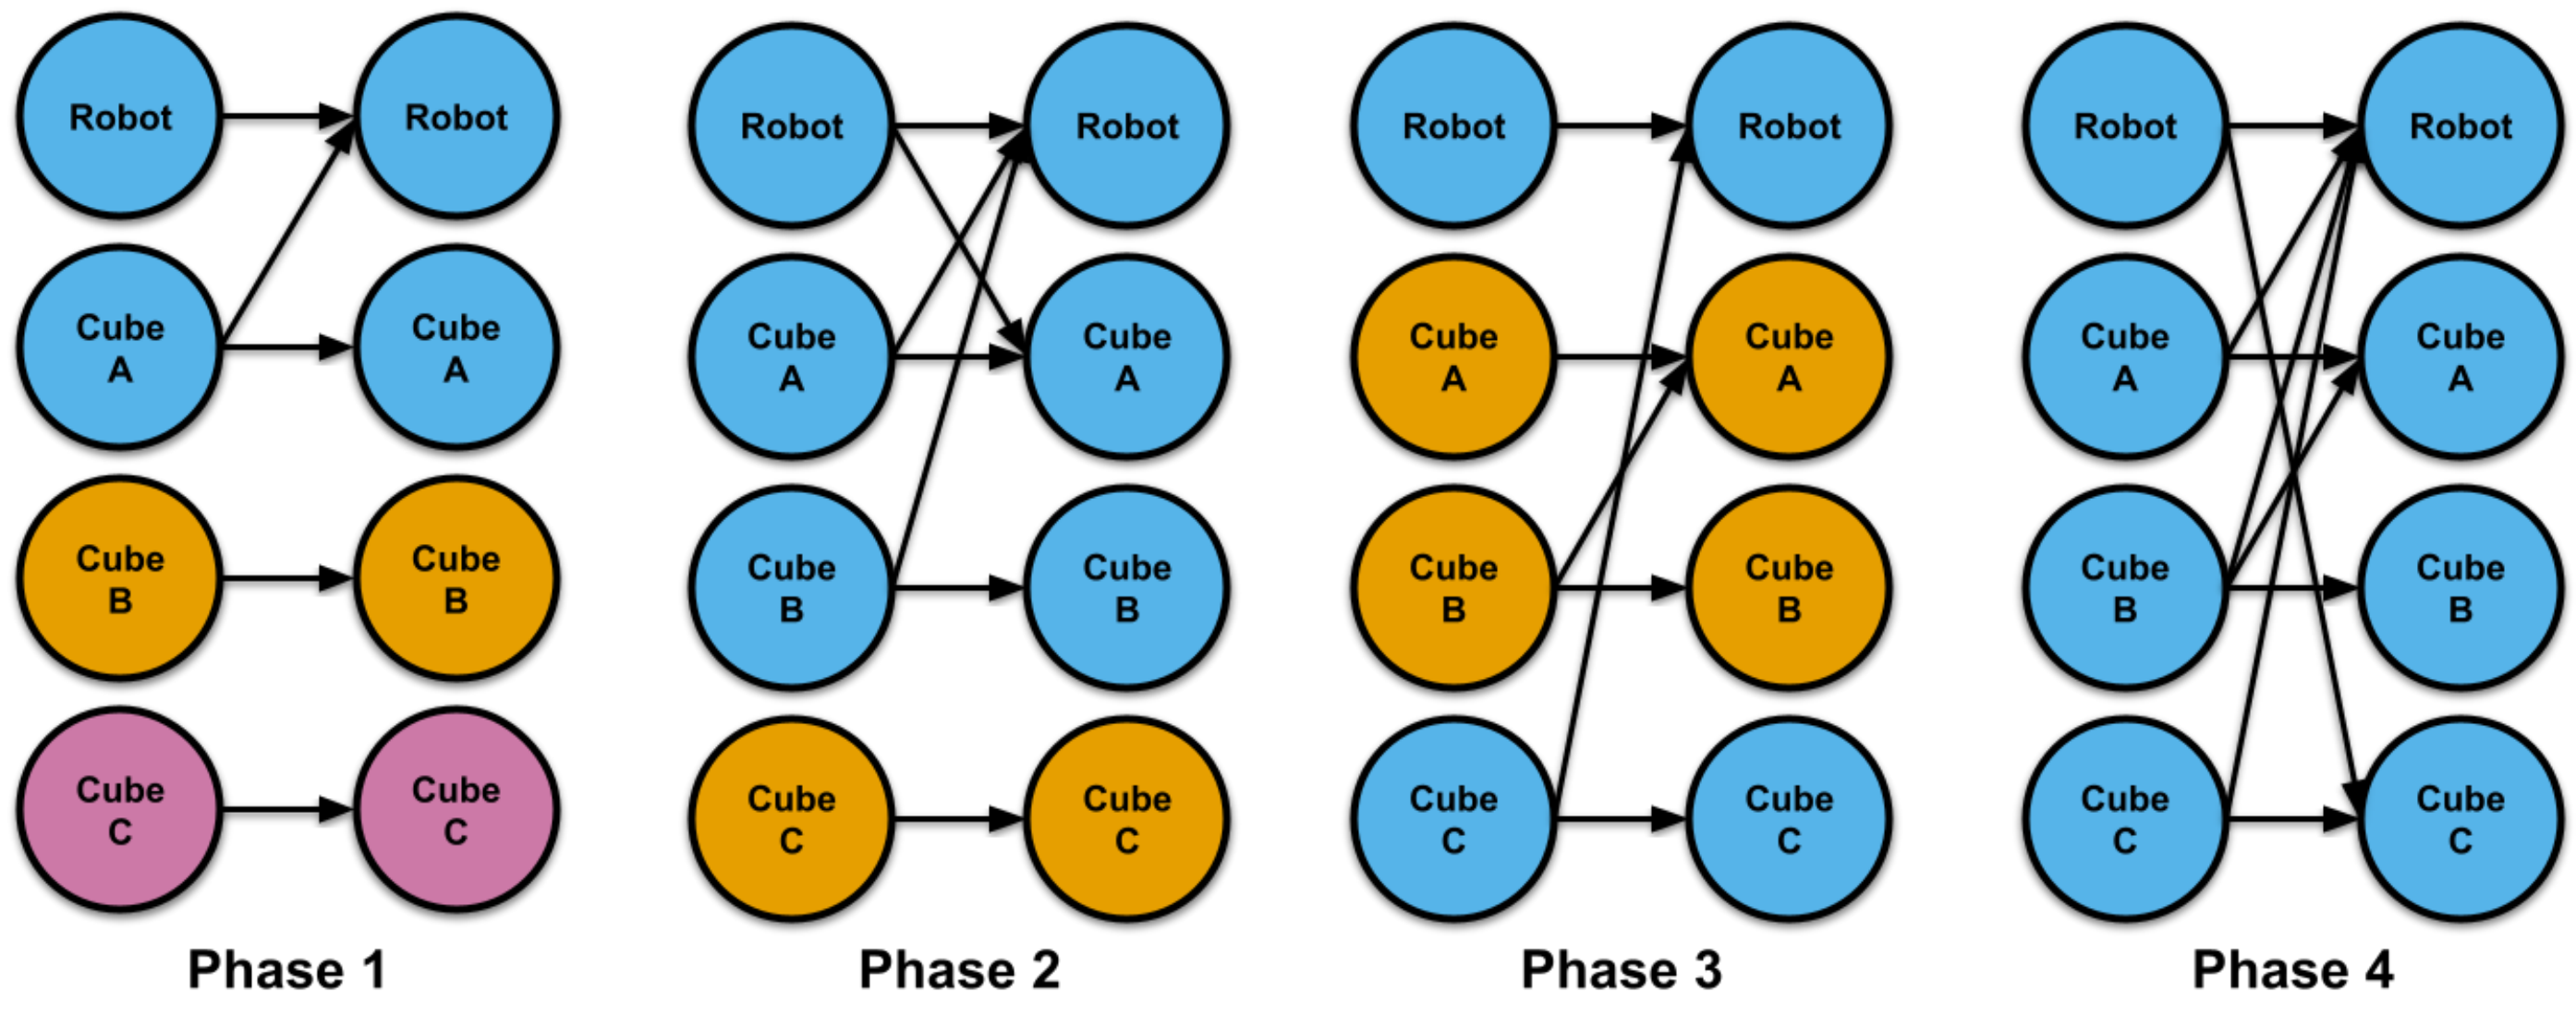}
    }
    \hfill
    \subfloat[Causal Graph of Coffee]{%
        \includegraphics[width=0.45\linewidth]{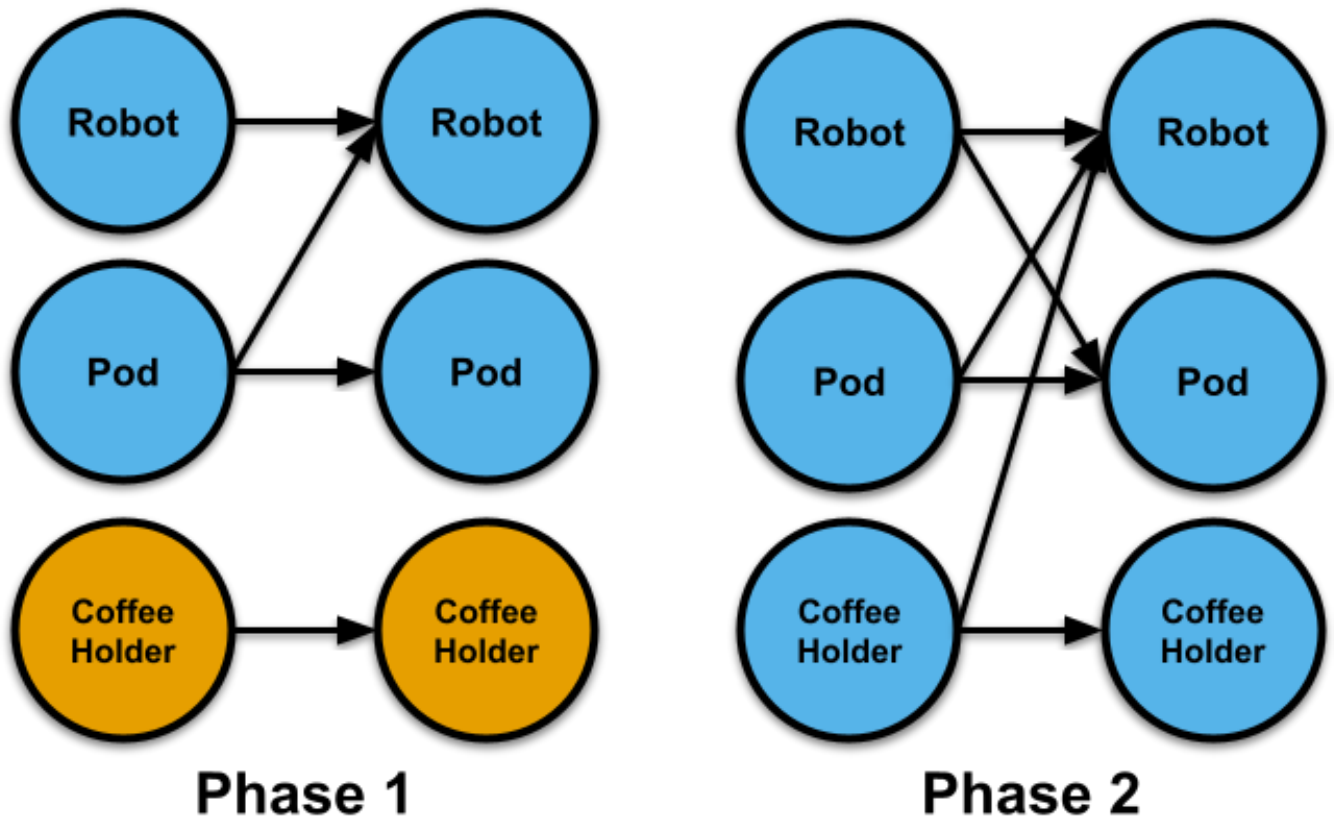}
    } 
    \caption{Causal relationships for each subtask. \textbf{(a)} \textit{Three Block Stack} has four subtasks: grasp cube A, place onto cube B, grasp cube C, place onto cubes A and B. Similarly \textit{Three Piece Assembly} follows the same general causal relationship as \textit{Three Block Stack}. \textbf{(b)} For \textit{Coffee}, there are two subtasks: grasp the coffee pod, then insert coffee pod into the holder before closing the lid. The colors represent partitions of independent entities where entities of the same color are causally dependent and entities of different colors are causally independent.}
    \label{fig:causalstack}
    % \vspace{-3mm}
\end{figure*}

\subsection{Scaling Synthetic Dataset Size}
We experiment with scaling the synthetic dataset size to understand the impact of data quantity on generalization. While data augmentation effectively increases the dataset and improves a model's generalization, there are diminishing returns. Similar to \cite{pitis2022mocoda} we explore increasing the dataset size and assess the ratio of demonstration data to causally augmented data. Separate from Section \ref{sec:CoDAaug} where data is sampled with some probability of applying causal augmentation, we augment offline as described in Algorithm \ref{alg:offlineCoDA}.

The performance of scaling the dataset is evaluated on \textit{Three Block Stack} and \textit{Coffee} using the same hyperparameters. We produce 500 demonstrations for each environment using $SE(3)$ equivariant data augmentation, expand the data up to 10x through causal augmentation, and train using the number of gradient steps fixed at one million. We report our performance as the maximum success rate for all policy evaluations on 3 separate seeds as done in \cite{mandlekar2021matters}. In the \textit{Three Block Stack} environment, performance improves by approximately $20\%$ when adding synthetic data up to a ratio of 1:1 (Figure \ref{fig:ratio}). However, as the dataset is expanded beyond the 1:1 ratio, the performance gains diminish with success rates falling within the margin of error. This indicates that adding more synthetic data beyond a 1:1 ratio does not result in substantial improvement and suggests some flexibility in the synthetic-to-real ratio. In certain tasks, we observed that counterfactual data augmentation sometimes led to out-of-distribution samples that reduced performance, especially at higher synthetic ratios (e.g., 1:5 in \textit{Coffee}). This may be attributed to the model’s sensitivity to shifts in the distribution when synthetic data dominates. Similarly, this aligns with discussion of \textbf{RQ3} in Section \ref{sec:experiments} as \textit{Three Block Stack} benefits largely from augmentation while \textit{Coffee} has marginal performance gains. We again attribute this to the complexity of each task -- notice that there are a total of 8 causally independent state partitions throughout the execution of \textit{Three Block Stack}, compared to only 2 for \textit{Coffee}.
% \subsection{Additional Experiments on Transport}
% We perform additional experiments on \textit{Transport} with four camera views (Table \ref{tab:transportaug4}). We show increasing the visual information increases the baseline performance and highlight Counterfactual Augmentation consistently outperforms other augmentations even with increased visual information.

% \begin{table}[!b]
% \centering
% \scriptsize % or \tiny for even smaller font
% \resizebox{0.70\columnwidth}{!}{% Resizes the table to fit within the column width
% \begin{tabular}{l|c} \hline
%     \toprule
%     \rowcolor[HTML]{CBCEFB} 
%     Augmentation Type& Success Rate (\%) \\ %\hline
%     \midrule
%     No Augmentation & 79\\ %\hline
%     \rowcolor[HTML]{EFEFEF} 
%     Channel Permutation & 92\\ %\hline
%     Color Jitter & 83\\ %\hline
%     \rowcolor[HTML]{EFEFEF} 
%     Priprioception Noise &84\\ %\hline
%     Random Resize \& Crop &90\\ %\hline        
%     \rowcolor[HTML]{EFEFEF} 
%     Counterfactual Augmentation &\textbf{94}\\ %\hline
%     % \rowcolor[HTML]{EFEFEF} 
%     % - CAR & & & &\\ %\hline
%     \bottomrule
% \end{tabular}
% }
% \caption{ACT policy performance on \texttt{Transport} using four camera views.}
% % \vspace{2mm}
% \label{tab:transportaug4}
% \vspace{-3mm}
% \end{table}
